# Supplementary material for: Slowly Quenched, High Pressure Glassy B$_2$O$_3$ at DFT Accuracy
Source: arXiv:2409.14949 ancillary file (2024-09-23)
Supplement: Supplementary file 1 [file Supporting_info.pdf]

## Supporting Information:

# Slowly Quenched, High-Pressure Glassy $B_2O_3$ at DFT Accuracy

Debendra Meher,[1] Nikhil V. S. Avula,[1] and Sundaram Balasubramanian[1]

*Chemistry and Physics of Materials Unit, Jawaharlal Nehru Centre for Advanced Scientific Research, India*

(Dated: 23 September 2024)

## CONTENTS

**S1. MLP Development** S3

A. Classical Force Field S3

B. Sampling Frames S5

C. MLP Training S7

D. MLP Testing S8

**S2. Comparison with AIMD** S8

**S3. Pressure-density data fit** S13

**S4. High Pressure B-O-B Angle** S14

**S5. System Size Dependence** S15

**References** S19

## S1. MLP DEVELOPMENT

The development of the machine-learned potential (MLP) requires the generation of several thousand configurations of $B_2O_3$ which should span all possible environments of the boron and oxygen atoms and various motifs of the glassy network. Next-neighbor structure of a particular atom type present in a glass, even at a particular state point, can vary across the substance. Furthermore, boron's coordination number (and geometry) changes with pressure. These call for a systematic consideration of many configurations in the training set.

In the initial versions of the MLP, such configurations are obtained from classical MD simulations carried out with the empirical potential[15]. These initial MD simulations with the classical potential were invariably performed at low density, around 1.5g/cc, and a temperature of 1600 K. Later, with the progressive refinement of the MLP, newer frames from the DPMD trajectory (i.e., the MD trajectory generated using the MLP) were added to the training dataset. As mentioned in the main text, all the frames from classical MD simulations were discarded at and beyond MLP version #20, and only frames from these DPMD simulations were retained in later datasets, including the final one, MLP-26.

In the following, we describe the empirical force field used herein for completeness.

### A. Classical Force Field

The interaction between boron and oxygen atoms of $B_2O_3$ was described using the potential of Wang et al. [15], which has been successfully used for the modeling of alkali borosilicate glasses. Its form is

$$U_{\mathbf{Buck}} = Ae^{-\frac{r}{B}} - \frac{C}{r^6} + \frac{z_1 z_2}{r} \tag{S1}$$

This force field yields a B-O bond length of 1.4 Å very close to that reported in experiments. It can also capture the transformation of three-coordinated boron atoms to four-coordinated ones upon the introduction of alkali oxide. Table S1 displays the force field parameters of Wang et al. [15] for the sake of completeness.

| Pair | A (kcal/mol) | B (Å) | C (kcal·Å$^6$/mol) |
|---|---|---|---|
| B-B | 11170.5294 | 0.350 | 0.0 |
| O-O | 208071.224 | 0.265 | 1962.27772 |
| B-O | 4772206.15 | 0.124 | 807.162989 |

TABLE S1. Force field parameters of Wang et al[15]. The charge on boron and oxygen are 1.4175e and -0.945e, respectively.

A spherical cutoff of 11 Å was applied to evaluate the total potential energy of the system through this potential. Long-range interactions were treated using the particle-particle particle mesh (PPPM) method with an accuracy of $10^{-5}$.

As the system modeled with this potential was quite viscous even at 1600 K, we needed to estimate the time taken for structural relaxation to determine the run lengths required for equilibration; thus, we examined the mean square displacement (MSD) of boron and oxygen at 1600 K. We noted that the linear displacement of the atoms over one ns was just 0.1 nm, as shown in Figure S1, which indicates that the atoms are not moving at all, even at 1600 K.

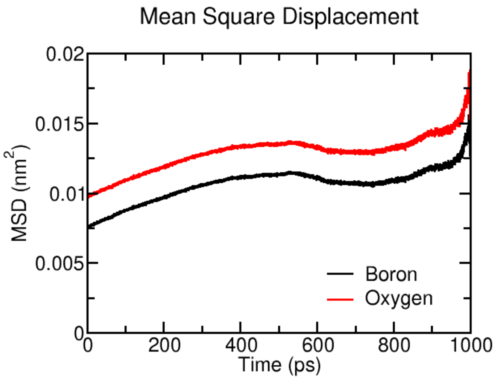


FIG. S1. Mean square displacement (MSD) of boron and oxygen in $B_2O_3$ modeled with the classical force field[15] at 1600 K and 1.502 g/cc.

### B. Sampling Frames

Since $B_2O_3$ modeled with the force field is highly viscous even at 1600 K, conducting a long molecular dynamics simulation to sample the phase space will not yield the uncorrelated frames required for the training set. To address this, we performed 200 independent MD runs with the force field using different initial configurations generated by PACKMOL with random seeds. These runs were started at a temperature of 3000 K followed by a ramping down of temperature to 1600 K at constant volume conditions, over 200 ps. Subsequently, we carried out production runs at 1600 K for 200 ps under constant NVT conditions, each at a density of 1.502 g/cc. The training dataset included frames from these runs and a few frames from MD trajectories conducted at 3000 K under constant NPT conditions. Additionally, we generated coordinates at densities of 1.502 g/cc $\pm$ 5% (i.e., at 5% higher and 5% lower densities than 1.502 g/cc) to sample configurations with different density values by rescaling the coordinates. Thus, 200 additional frames were added to the training

set.

In this manner, we collected around 2000 frames from these classical MD trajectories (1600 K-3000 K at 1 bar) to train the MLP model in six stages. After the sixth version of the MLP, we started the iterative training of MLPs using frames sampled from exploratory MD simulations of previous MLP generations. Subsequently, we trained 14 MLP generations and obtained the 20th generation of MLP, consisting of 15400 frames generated from simulations whose temperatures ranged from 5 K to 3000 K and pressures from 0 to 5 GPa. In the penultimate stages of MLP development, we removed the frames contributed by classical MD simulations, a few redundant ones, and a few outliers. In Table S2, we provide a summary of the frames constituting the training dataset of MLP-26. Table S3 demonstrates the accuracy of the MLP models for different model hyperparameters.

**Single point energy calculations:** We utilized a Double-Zeta Valence and Polarization MOLOPT with Short Range (DZVP-MOLOPT-SR) basis set. We have chosen EPS_DEFAULT, which controls several thresholds in the SCF procedure of CP2k[7] as $10^{-14}$.

## C. MLP Training

| index | Ensemble | Temperature (K) | Pressure (GPa) | Frames |
|---|---|---|---|---|
| 1 | NVT | 5-1600 | 0 | 200 |
| 2 | NVT | 1600 | 0 | 400 |
| 3 | NVT | 1600-3000 | 0 | 399 |
| 4 | NVT | 3000 | 0 | 789 |
| 5 | NPT | 3000 | 0 | 690 |
| 6 | NPT | 3000 | 0-1 | 589 |
| 7 | NPT | 3000 | 1 | 985 |
| 8 | NPT | 1600 | 0 | 400 |
| 9 | NPT | 1600-300 | 0 | 400 |
| 10 | NPT | 300 | 0-1 | 720 |
| 11 | NPT | 300 | 1-10 | 419 |
| 12 | NPT | 300 | 10-50 | 1223 |
| 13 | NPT | 300 | 50-100 | 740 |
| 14 | NPT | 300 | 100-200 | 1000 |
| 15 | NPT | 300 | 100-500 | 100 |
| Total | NVT and NPT | 5 K to 3000 K | 0-500 | 9625 |

TABLE S2. Dataset constituting the final MLP generation, MLP-26, used in the manuscript. These frames were obtained using DPMD through an iterative procedure described in the main text.

### D. MLP Testing

Most of the hyperparameters of the DP models used in this work were similar to that of the standard values in the literature[2,14,16]. We investigated the effect of two hyperparameters - $r_s$ and the number of training steps - which seem to depend on the specific system. Table S3 summarizes the results of the hyperparameter tuning study. The $r_s$ (distance from which the smoothing function starts acting on the descriptor[16]) value of 0.5 Å shows a significant improvement in the performance of the MLPs over the default value of 5.8 Å. Hence, we adopted the value of 0.5 Å for the final MLP. The study also shows that the number of training steps does not change the performance significantly beyond two million steps.

| $r\_smt$ | Training steps($10^6$) | Energy RMSE (meV) | | Force RMSE (meV/Å) | |
|---|---|---|---|---|---|
| | | Training | Validation | Training | Validation |
| 5.8 | 2 | 3.4 | 3.4 | 270 | 282 |
| 0.5 | 2 | 2.4 | 2.5 | 221 | 240 |
| 0.5 | 4 | 2.3 | 2.4 | 216 | 235 |
| 0.5 | 6 | 2.2 | 2.3 | 213 | 234 |
| 0.5 | 8 | 2.1 | 2.3 | 211 | 231 |
| 0.5 | 10 | 2.2 | 2.3 | 211 | 232 |

TABLE S3. Accuracy of MLPs for different hyperparameters.

## S2. COMPARISON WITH AIMD

All the AIMD simulations were carried out using the Quickstep module of the CP2K simulation program. The revised version of the Perdew-Burke-Ernzerhof GGA

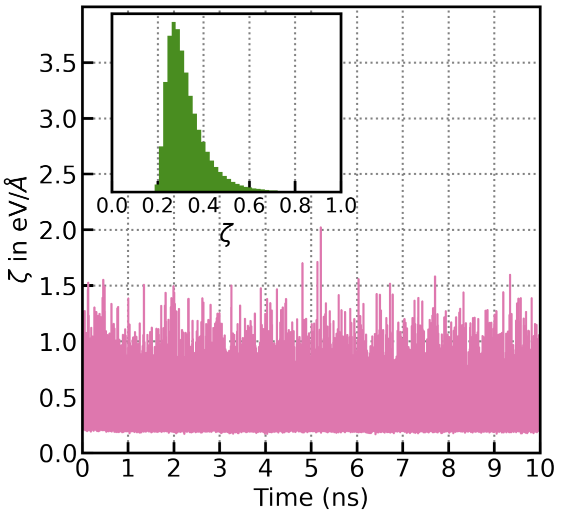


FIG. S2. Model deviation for $B_2O_3$ glass at 3.6 g/cc and 2400 K containing 265 atoms.

exchange-correlation functional was used to treat the valence electrons (revPBE-D3). Molecularly optimized Double-Zeta Valence and Polarization with Shorter Range (DZVP-MOLOPT-SR) basis set was used for B/O atoms. The core electrons were treated with Goedecker-Teter-Hutter (GTH) norm-conserving pseudopotentials. Grimme's D3 empirical correction term with a cutoff of 40 Å was also used. We note that the configurations sampled for training and validation sets had their single point energy (SPE) calculations done using an energy cutoff of 1200 Ry. Figure S3 displays the convergence of energy with this cutoff value. The trajectory was evolved using the Born-Oppenheimer molecular dynamics scheme with a timestep of 1 fs. NVT simulations were carried out at two different temperatures, 1600 K and 2000 K (at both these temperatures, $B_2O_3$ is in liquid state experimentally). The thermostat time constant was set to be 100 fs corresponding to 3000 $cm^{-1}$. The total trajectory was run for 20 ps, and the last ten ps were used to analyze the results. The production run of AIMD-2 was 30 ps long with a 10 ps equilibration.

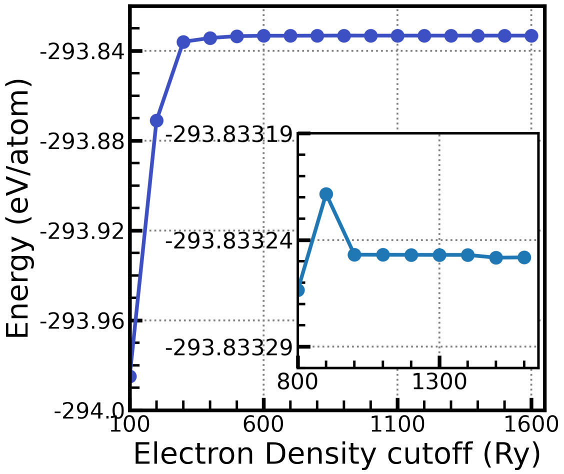


FIG. S3. Energy convergence test for DFT total energy calculation by varying the energy cutoff. Inset shows the zoomed-in version of the same for large cutoff values.

In the main manuscript, we noted (Figure 3) that the RDFs and bond angle distributions obtained from DPMD simulations at 2000 K matched those obtained from two independent AIMD simulations. To further support the fidelity of the MLP-26 and DPMD, which uses the same, we have carried out two additional AIMD simulations at 1600 K. These results are compared against those from a DPMD simulation performed under the same conditions in Figure S4 and Figure S5. The AIMD and DPMD results match very well, offering further confirmation of the accuracy of MLP-26.

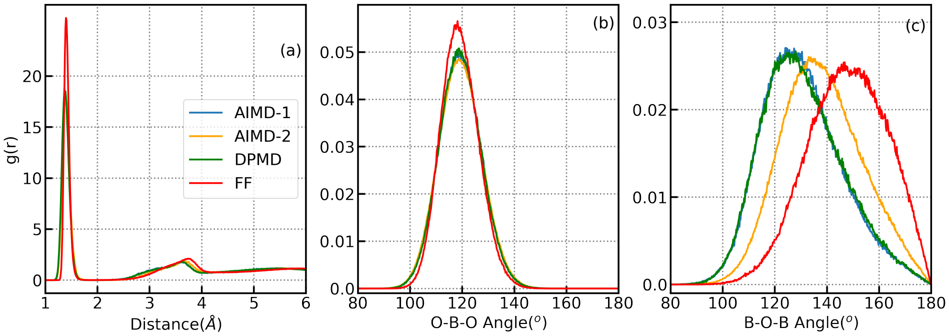


FIG. S4. Comparison of DPMD results against those from two AIMD simulations started from different initial configurations, all performed at 1.502 g/cc and 1600 K. Results from empirical force field-based MD simulations are also compared. (a) B-O RDF (b) O-B-O angle distribution (c) B-O-B angle distribution. The AIMD simulation, whose result is shown in orange (AIMD-2), was started from a configuration equilibrated with the force field, whose distribution is in red. On the other hand, the AIMD-1 simulation was started from a configuration equilibrated by DPMD. In panel (c), the orange curve does not overlap with the results of either DPMD or of AIMD-1 due to the short duration of the trajectory (40 ps).

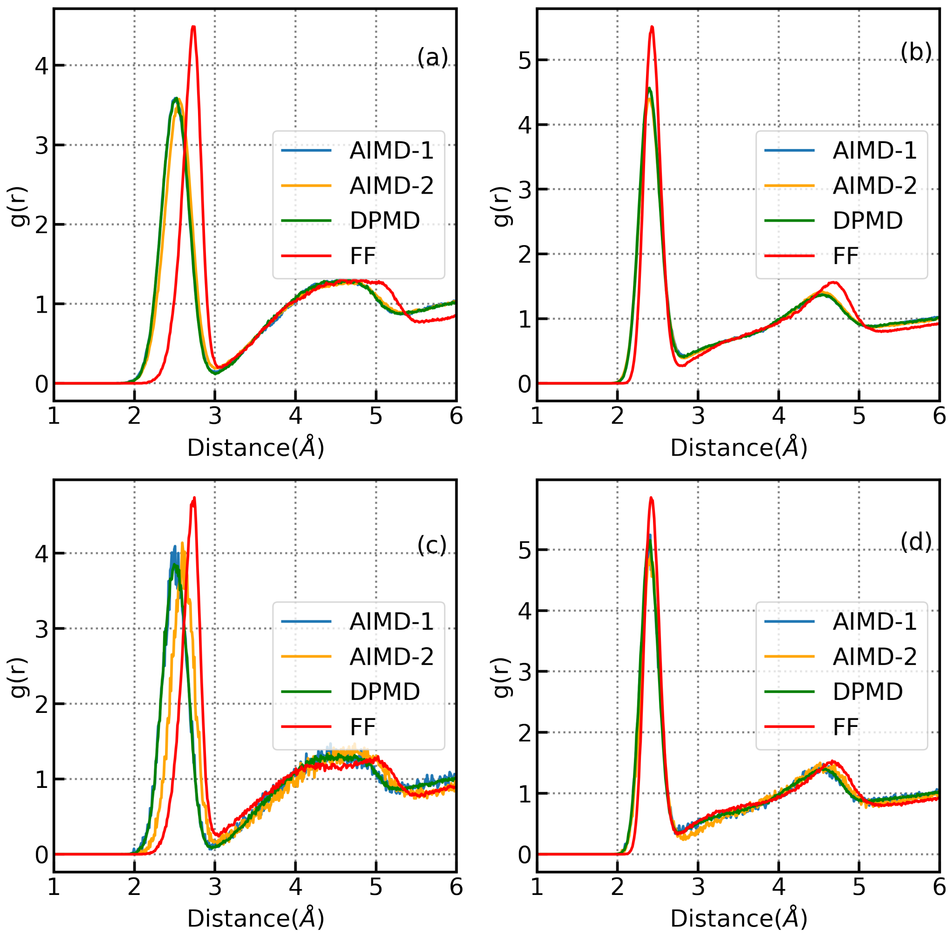


FIG. S5. Comparison of B-B and O-O RDFs from DPMD and the two independent AIMD runs at two conditions: 1600 K (and 1.502 g/cc) and 2000 K (and 1.49 g/cc).

Further, unlike the $B_2O_3$ modeled with the classical force field, the one studied with MLP-26 displays an adequate sampling of configurations in the melt. In Fig-

ure S6, we show the distinct part of the van Hove correlation function of $B_2O_3$ at 2400 K and a high density of 3.2 g/cc. It is seen that the correlation function decorrelates to a uniform value of unity within a few tens of picoseconds. The faster structural relaxation of $B_2O_3$ in the MLP-26 description is also observed in the diffusion coefficients of the atoms. Figure S7 compares the mean square displacement of atoms at three temperatures between the force field and the MLP descriptions.

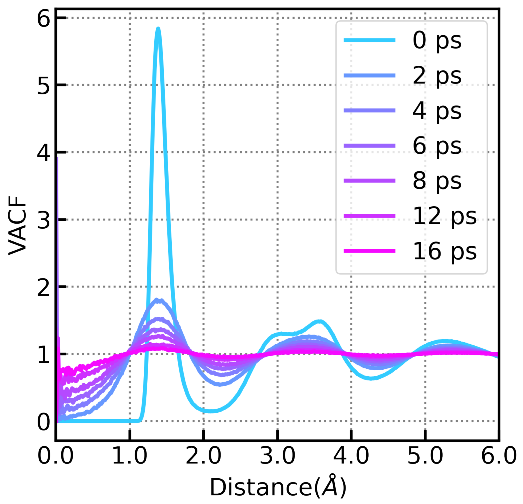


FIG. S6. Distinct part of the B-O van Hove space-time correlation function at 3.2 g/cc density and 2400 K temperature.

## S3. PRESSURE-DENSITY DATA FIT

The experimental pressure vs. density[1] as well as the pressure-density data from our DPMD simulations were fitted to third-order polynomials S2. The dependence

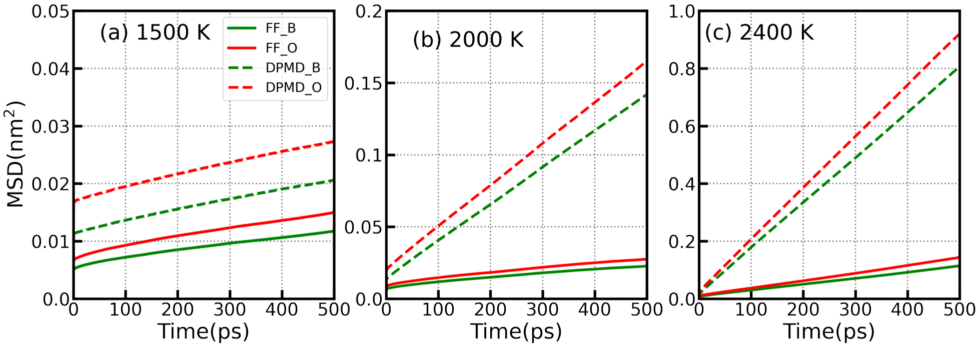


FIG. S7. Comparison of mean squared displacement of atoms from MD trajectories generated with the force field[15] and from the DPMD run. The density in all the three systems is 1.844 g/cc.

of glass density on the quenching rate (Inset II of Figure 4) was thus obtained.

$$y = ax^3 + bx^2 + cx + d \tag{S2}$$

## S4. HIGH PRESSURE B-O-B ANGLE

In the main manuscript, in Figure 10a, we presented the distribution of B-O-B angles at various densities of the $B_2O_3$ glass. The distribution at 2.854 g/cc developed a small peak at $90^o$ which was attributed to four-membered rings. We have ascertained that this feature is intrinsic and does not show any systematic dependence on the quenching rate in Figure S8.

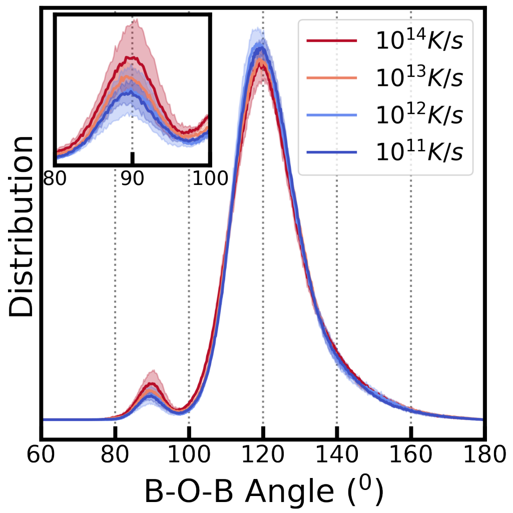


FIG. S8. Distribution of B-O-B angle in $B_2O_3$ glass at 2.854 g/cc obtained at various quenching rates. Inset shows the same around an angle of $90^o$.

## S5. SYSTEM SIZE DEPENDENCE

The results presented in the main manuscript pertain to a system size of 1700 atoms (340 $B_2O_3$ units). However, typical AIMD simulations of glasses only have a few hundred atoms. In this section, we provide results of DPMD simulations for $B_2O_3$ containing 360 atoms. The results shown in the main manuscript with 1700 atoms (particularly on the dependence of density on the quenching rate, the artifactual four-membered ring seen at high quenching rates, etc.) are all observed at the smaller system size as well, demonstrating the robustness of the results. The distribution of ring sizes shows an abrupt drop in glassy $B_2O_3$ modeled with 360 atoms (Figure S11), in comparison to the smooth decay to zero for the one modeled with 1700 atoms (Figure 11).

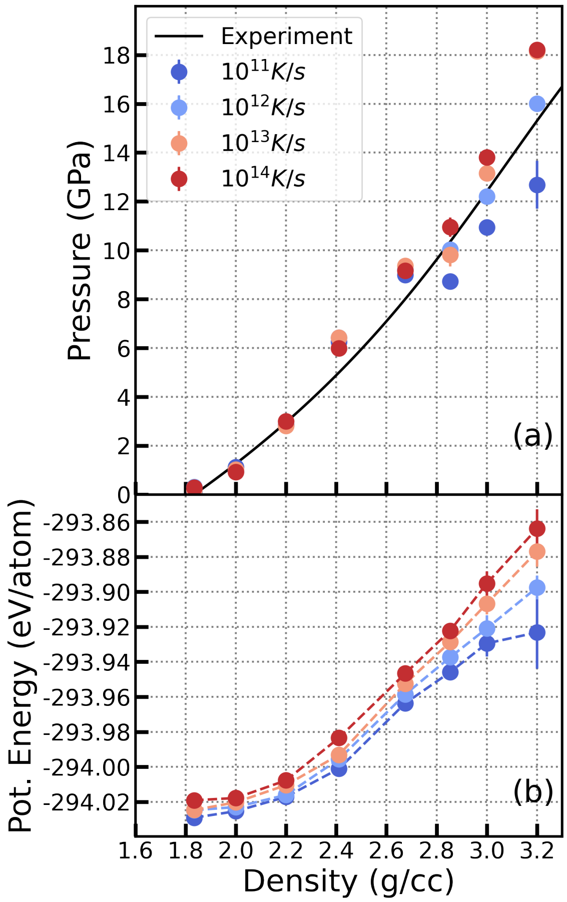


FIG. S9. Pressure vs density and pressure vs potential energy for 360 atoms.

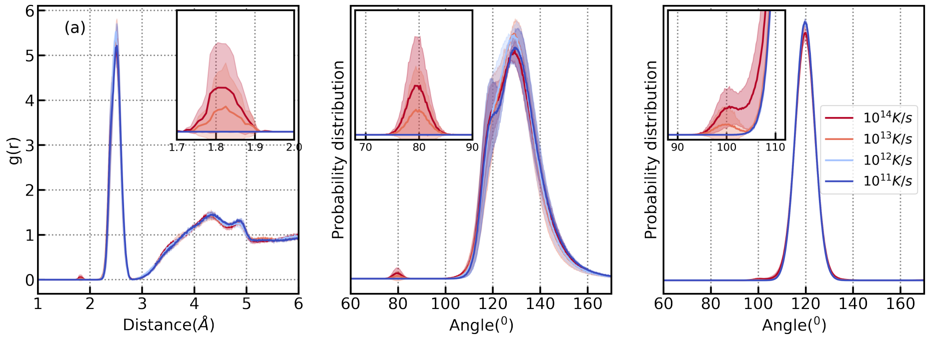


FIG. S10. Effect of quenching rate on the glass structure at 300 K and 1.834 g/cc density for 360 atoms. (a) B-B RDF shows a small peak at a distance of less than 2 Å at high quenching rates. Its height decreases with a decreasing quenching rate, and the peak vanishes at the slowest quenching rate of $10^{11}$ K/s. (b) B-O-B bond angle distribution displays a hump at 80° for high quenching rates, which is the angle formed at the oxygen atom in a four-membered ring (B-O-B-O) with a boron-boron distance of around 1.8 Å. (c) the bond angle distribution of O-B-O also shows a peak at 100° due to a few four-membered rings formed as an artifact at high quenching rates; the same is absent at the slowest quenching rate. Insets in all the panels show the zoomed-in region around this artifact.

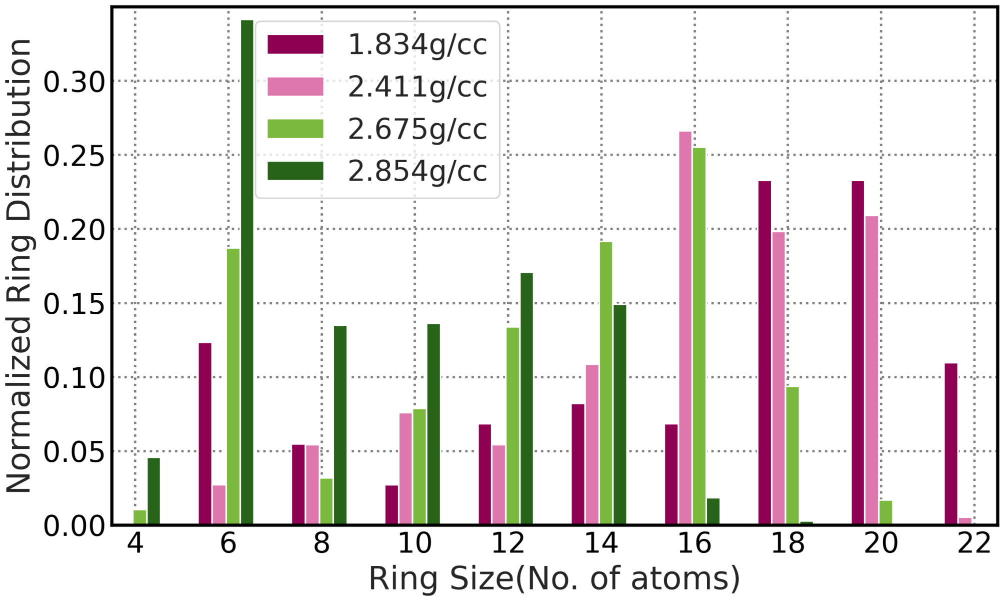


FIG. S11. Ring size distribution in $B_2O_3$ glasses at different densities. For 360 atoms, there is an abrupt cutoff after ring size 22 for the lowest density due to the small box size. With increasing density, the fraction of smaller rings increases.

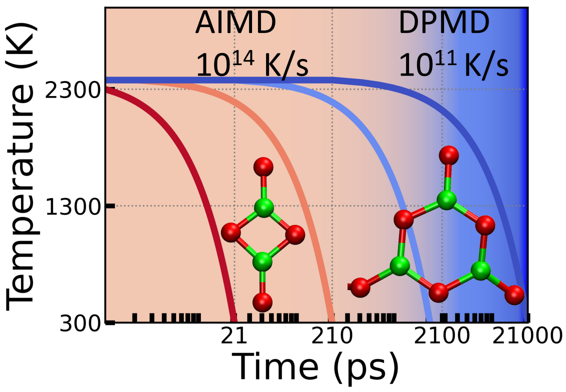


FIG. S12. Highlight Image

## REFERENCES

[1] V. V. Brazhkin, Y. Katayama, K. Trachenko, O. B. Tsiok, A. G. Lyapin, E. Artacho, M. Dove, G. Ferlat, Y. Inamura, and H. Saitoh. Nature of the structural transformations in $b_2o_3$ glass under high pressure. *Phys. Rev. Lett.*, 101:035702, Jul 2008. doi:10.1103/PhysRevLett.101.035702.

[2] N. M. Chtchelkatchev, R. E. Ryltsev, M. V. Magnitskaya, S. M. Gorbunov, K. A. Cherednichenko, V. L. Solozhenko, and V. V. Brazhkin. Local structure, thermodynamics, and melting of boron phosphide at high pressures by deep learning-driven ab-initio simulations. *The Journal of Chemical Physics*, 159:064507, 08 2023. ISSN 0021-9606. doi:10.1063/5.0165948.

[3] H. Dong, A. R. Oganov, V. V. Brazhkin, Q. Wang, J. Zhang, M. M. Davari Esfahani, X.-F. Zhou, F. Wu, and Q. Zhu. Boron oxides under pressure: Prediction of the hardest oxides. *Phys. Rev. B*, 98:174109, Nov 2018. doi:10.1103/PhysRevB.98.174109. URL `https://link.aps.org/doi/10.1103/PhysRevB.98.174109`.

[4] S. Goedecker, M. Teter, and J. Hutter. Separable dual-space gaussian pseudopotentials. *Phys. Rev. B*, 54:1703–1710, Jul 1996. doi:10.1103/PhysRevB.54.1703. URL https://link.aps.org/doi/10.1103/PhysRevB.54.1703.

[5] S. Grimme, J. Antony, S. Ehrlich, and H. Krieg. A consistent and accurate ab initio parametrization of density functional dispersion correction (DFT-D) for the 94 elements H-Pu. *The Journal of Chemical Physics*, 132(15):154104, 04 2010. ISSN 0021-9606. doi:10.1063/1.3382344. URL https://doi.org/10.1063/1.3382344.

[6] C. Hartwigsen, S. Goedecker, and J. Hutter. Relativistic separable dual-space gaussian pseudopotentials from h to rn. *Phys. Rev. B*, 58:3641–3662, Aug 1998. doi:10.1103/PhysRevB.58.3641. URL https://link.aps.org/doi/10.1103/PhysRevB.58.3641.

[7] T. D. Kühne, M. Iannuzzi, M. Del Ben, V. V. Rybkin, P. Seewald, F. Stein, T. Laino, R. Z. Khaliullin, O. Schütt, F. Schiffmann, D. Golze, J. Wilhelm, S. Chulkov, M. H. Bani-Hashemian, V. Weber, U. Borštnik, M. Taillefumier, A. S. Jakobovits, A. Lazzaro, H. Pabst, T. Müller, R. Schade, M. Guidon, S. Andermatt, N. Holmberg, G. K. Schenter, A. Hehn, A. Bussy, F. Belleflamme, G. Tabacchi, A. Glöß, M. Lass, I. Bethune, C. J. Mundy, C. Plessl, M. Watkins, J. VandeVondele, M. Krack, and J. Hutter. CP2K: An electronic structure and molecular dynamics software package - Quickstep: Efficient and accurate electronic structure calculations. *The Journal of Chemical Physics*, 152(19):194103, 05 2020. ISSN 0021-9606. doi:10.1063/5.0007045. URL https://doi.org/10.1063/5.0007045.

[8] S. K. Lee, P. J. Eng, H.-k. Mao, Y. Meng, M. Newville, M. Y. Hu, and J. Shu. Probing of bonding changes in b2o3 glasses at high pressure with inelastic x-ray scattering. *Nature Materials*, 4(11):851–854, Nov 2005. ISSN 1476-4660. doi:10.1038/nmat1511. URL https://doi.org/10.1038/nmat1511.

[9] J. M. Martínez and L. Martínez. Packing optimization for automated generation of complex system's initial configurations for molecular dynamics and

docking. *Journal of Computational Chemistry*, 24(7):819–825, 2003. doi: https://doi.org/10.1002/jcc.10216. URL https://onlinelibrary.wiley.com/doi/abs/10.1002/jcc.10216.

[10] L. Martínez, R. Andrade, E. G. Birgin, and J. M. Martínez. Packmol: A package for building initial configurations for molecular dynamics simulations. *Journal of Computational Chemistry*, 30(13):2157–2164, 2009. doi: https://doi.org/10.1002/jcc.21224. URL https://onlinelibrary.wiley.com/doi/abs/10.1002/jcc.21224.

[11] D. Nieto-Sanz, P. Loubeyre, W. Crichton, and M. Mezouar. X-ray study of the synthesis of boron oxides at high pressure: Phase diagram and equation of state. *Phys. Rev. B*, 70:214108, Dec 2004. doi:10.1103/PhysRevB.70.214108. URL https://link.aps.org/doi/10.1103/PhysRevB.70.214108.

[12] M. M. Smedskjaer, R. E. Youngman, S. Striepe, M. Potuzak, U. Bauer, J. Deubener, H. Behrens, J. C. Mauro, and Y. Yue. Irreversibility of pressure induced boron speciation change in glass. *Scientific Reports*, 4(1):3770, Jan 2014. ISSN 2045-2322. doi:10.1038/srep03770. URL https://doi.org/10.1038/srep03770.

[13] A. P. Thompson, H. M. Aktulga, R. Berger, D. S. Bolintineanu, W. M. Brown, P. S. Crozier, P. J. in 't Veld, A. Kohlmeyer, S. G. Moore, T. D. Nguyen, R. Shan, M. J. Stevens, J. Tranchida, C. Trott, and S. J. Plimpton. Lammps - a flexible simulation tool for particle-based materials modeling at the atomic, meso, and continuum scales. *Computer Physics Communications*, 271:108171, 2022. ISSN 0010-4655. doi: https://doi.org/10.1016/j.cpc.2021.108171. URL https://www.sciencedirect.com/science/article/pii/S0010465521002836.

[14] H. Wang, L. Zhang, J. Han, and W. E. Deepmd-kit: A deep learning package for many-body potential energy representation and molecular dynamics. *Computer Physics Communications*, 228:178–184, 2018. ISSN 0010-4655. doi:

https://doi.org/10.1016/j.cpc.2018.03.016. URL https://www.sciencedirect.com/science/article/pii/S0010465518300882.

[15] M. Wang, N. Anoop Krishnan, B. Wang, M. M. Smedskjaer, J. C. Mauro, and M. Bauchy. A new transferable interatomic potential for molecular dynamics simulations of borosilicate glasses. *Journal of Non-Crystalline Solids*, 498:294–304, 2018. ISSN 0022-3093. doi:https://doi.org/10.1016/j.jnoncrysol.2018.04.063. URL https://www.sciencedirect.com/science/article/pii/S0022309318302643.

[16] J. Zeng, D. Zhang, D. Lu, P. Mo, Z. Li, Y. Chen, M. Rynik, L. Huang, Z. Li, S. Shi, Y. Wang, H. Ye, P. Tuo, J. Yang, Y. Ding, Y. Li, D. Tisi, Q. Zeng, H. Bao, Y. Xia, J. Huang, K. Muraoka, Y. Wang, J. Chang, F. Yuan, S. L. Bore, C. Cai, Y. Lin, B. Wang, J. Xu, J.-X. Zhu, C. Luo, Y. Zhang, R. E. A. Goodall, W. Liang, A. K. Singh, S. Yao, J. Zhang, R. Wentzcovitch, J. Han, J. Liu, W. Jia, D. M. York, W. E, R. Car, L. Zhang, and H. Wang. DeePMD-kit v2: A software package for deep potential models. *The Journal of Chemical Physics*, 159:054801, 08 2023. ISSN 0021-9606. doi:10.1063/5.0155600.

[17] Y. Zhang and W. Yang. Comment on "generalized gradient approximation made simple". *Phys. Rev. Lett.*, 80:890–890, Jan 1998. doi:10.1103/PhysRevLett.80.890. URL https://link.aps.org/doi/10.1103/PhysRevLett.80.890.
